# Supplementary material for: The Loopix Anonymity System
Source: arXiv:1703.00536 source file (2017-03-01)
Supplement: Supplementary file 1 [file appendix_proof.tex]

%!Tex root = ../loopix.tex

\newcommand{\chal}{\ensuremath{\mathrm{Ch}}\xspace}
\newcommand{\ano}{\ensuremath{\alpha}\xspace}
\newcommand{\eps}{\ensuremath{\varepsilon}\xspace}
\newcommand{\Exp}{\ensuremath{\mathsf{Exp}}\xspace}
\newcommand{\interact}[2]{\ensuremath{\langle #1 \mid #2 \rangle}\xspace}
\newcommand{\myparagraph}[1]{\textbf{#1}\quad}

\section{Postponed security proofs and notions}\label{sec:postponedproofs}
In this section we present a more precise definition of Loopix anonymity against the global passive adversary (GPA) that might collaborate with local passive adversaries, e.g., honest but curious mix servers. To this end we use the AnoA framework~\cite{backes2013anoa} for defining anonymity in terms of a computational indistinguishability notion.

\subsection{Loopix in AnoA}

\begin{definition}[Adversary's Advantage]\label{def:anonymity}
Let $\ano$ be an anonymity function,  $\gamma \in \mathbb{N}$. Then, the \emph{adversary's advantage} of an adversary $\adv$ against Loopix for $\gamma$ challenges of the anonymity notion $\ano$ is bounded by $\eps$ and $\delta$, with $\eps \geq 0, 0 \leq \delta \leq 1$,  if for all sufficiently large $\eta\in\mathbb{N}$, we have
\[
\begin{aligned}
					&\pr{0 = \interact{\adv(1^\eta)}{\chal(\ano,\gamma,0)}} \\
\leq\ e^\eps\ &	 \pr{0 = \interact{\adv(1^\eta)}{\chal(\ano,\gamma,1)}} + \delta.
\end{aligned}
\]
We say that Loopix provides $\ano$ up to $\delta$.
\end{definition}

\myparagraph{Assumptions and abstractions}
We assume for our analysis that the implementation of the cryptographic primitives underlying the Loopix system is flawless. Moreover we abstract away the computational overhead, space restrictions and communication costs as well as timing channels of clients and mix servers and we assume that there is no network latency other than the delays imposed by Loopix. We abstractly describe what an observer can learn about messages and packets that are sent through Loopix as transmissions $(S,t,h,R)$, a tuple describing the immediate sender $S$ of a packet $h$, the time of transmission $t$ and the immediate recipient $R$ of the packet. Note that $t$ is also the time of arrival of the packet. 

We abstract away from compromised users in our analysis, as the adversary can simulate their behavior. For analyzing Loopix against passive adversaries we use the fact that packets are indistinguishable for an external adversary (c.f., \Cref{sec:message_indistinguishability}), to consider $h$ to be a handle that does not any information. Recipients of the handle can get the information embedded within it, which necessarily includes the next hop (for mix servers) or the payload (for recipients).

%More formally, for a set of possible transmissions $\transmissions$, we abstract away the game between the adversary and the challenger as randomly generating traces and observations, where a trace $\trace \in \transmissions^l$ is the consecutive observations an adversary could make for one particular message traversing the network. We say a trace $\trace = ((S_1,h_1,t_1,R_1), \ldots (S_l,h_l,t_l,R_l))$ is valid if $S_1$ is a user, $S_2$ is the provider of that user, and if for all $i \in \set{1, l-1}.\ R_i = S_{i+1} \land t_i < t_{i+1}$.

More formally, we define transitions and traces as follows.
\begin{definition}[Transmissions and traces]
A transmission $(S,t,h,R) \in \left(U \cup M \cup P\right) \times \mathbb N \times \mathbb R^+\times \left(U \cup M \cup P\right) =: \transmissions$ is a triple describing the immediate sender $S$ of a handle $h$, the time of transmission $t$ and the immediate recipient $R$ of the handle. We define a trace $\trace \in \transmissions^l$ as the consecutive observations an adversary can make for one particular message traversing the network. We say a trace $\trace = ((S_1,h_1,t_1,R_1), \ldots (S_l,h_l,t_l,R_l))$ is valid if $S_1 \in U, S_2 \in P, S_l \in P$ and if for all $i \in \set{1, l-1}.\ R_i = S_{i+1} \land t_i < t_{i+1}$.
\end{definition}

Based on transmissions and traces we can now define a simple abstraction of Loopix that allows for further reasoning about the properties of the network.

\begin{definition}[Simple Loopix]\label{def:simpleloopix}
All users and mix servers have access to a trusted third party (TTP) that is parametric in a set of corrupt mix servers $\mathsf{A}$. The idealized system only models drop messages and payload messages, not loops. Clients send drop messages by choosing a random provider $p$ and sending a special drop symbol and $p$ to the TTP. They send payload messages $m$ to a recipient $r$ hosted by provider $p$ by sending ($p$, $r$, $m$) to the TTP.  The TTP keeps track of a set of transmissions $O_T \subseteq \transmissions$, a set of all adversarial correlations of transmissions $O_CC \subseteq$, and a set $O_M$ of received messages and the times of their arrival to the recipient $(m,t) \in \set{0,1}^* \times \mathbb R$.

For every message sent by a client $u$ hosted at provider $p_u$ at time $t_1$ to a provider $p$, the TTP computes a trace $\trace = ((S_1,h_1,t_1,R_1), \ldots (S_l,h_l,t_l,R_l)) \in \transmissions^l$ such that $\trace$ is valid and $S_1 = u, R_1 = p_u$, $R_l = p$ and for $i \in \set{2, \ldots, l-1}. R_i$ is chosen uniformly at random from all mix nodes at layer $i$, $h_i \in \mathbb N$ is a fresh random nonce and $t_i = t_{i+1} + d$, where $d$ is sampled from the exponential distribution with parameter $\mu$. The TTP then adds all transmissions $t$ in $\trace$ to $O_T$ and for all $i \in \set{1, \ldots, l-1}$ s.t. $R_i \in \mathsf{A}$ the TTP adds $((S_i,h_i,t_i,R_i), (S_{i+1},h_{i+1},t_{i+1},R_{i+1}))$ to $O_C$. If the message is a payload message $m$, the TTP also adds $(m, t_l)$ to $O_M$. The TTP then secretly forwards the message to the recipient.

The challenger allows the adversary an oracle access to $(O_T, O_C, O_M)$, but only to elements with timestamps that don't lie in the future.
\end{definition}

\begin{theorem}[Soundness of Simple Loopix]\label{thm:simpleloopix}
If Simple Loopix, given the set $\mathcal A$ provides sender-receiver third party unlinkability up to $\delta$ against an adversary observing $(O_T, O_C, O_M)$ then Loopix provides sender-receiver third party unlinkability up to $\delta$ against a GPA that additionally (passively) compromises all mix servers in $\mathcal A$.
\end{theorem}
\begin{proof}

%\subsection{Proof of \Cref{thm:simpleloopix}}

\myparagraph{Recap - Anonymity Game}
We assume in the following that the adversary is playing the AnoA game against a challenger. The adversary chooses the behaviour of all users, excluding one challenge: At any time the adversary can send a message Challenge $(A,B,C,D, m_C, m_D)$ to the challenger which will either make $A$ send a message $m_C$ to $C$ and $B$ send a message $m_D$ to $D$ (if the challenge bit $b=0$), or it will make $A$ send a message $m_D$ to $D$ and $B$ send a message $m_C$ to $C$ (if the challenge bit $b=1$). The adversary wins the game if it correctly guesses the challenge bit $b$ after making its observations. Note that the adversary is a global passive adversary that can control the time at which the challenge is sent and that additionally observes all recipients.

\myparagraph{Proof Structure}
The proof will progress as a series of games. We will start with the actual Loopix protocol in the AnoA game as described above and will then gradually reduce the complexity in a sound way, showing that the adversarial success is preserved from one game to the next. 

\myparagraph{Notation}
With Game $i$ $\leq$ Game $i+1$ we describe that the adversarial advantage in Game $i$ is at least as large as the adversarial advantage in Game $i+1$. Analogously we write Game $i$ $\approx$ Game $i+1$ to describe that the adversarial advantage is the same up to a difference negligible in the security parameter.

\myparagraph{Game 0}
We begin the proof with the actual instantiation of Loopix, including the Sphinx packet format providing encryptions, group elements and other cryptographic aspects. In this game, as well as in any of the following games, the adversary chooses the payload messages of all users, except for the users $A$ and $B$, to whom he issues a  challenge message, as described above. Finally, in every game the adversary outputs a bit $b^*$ and wins if $b^* = b$.

\myparagraph{Game 1 (idealized cryptography)}
Instead of sending Sphinx packets, all protocol participants only send handles $h$ to each other instead of actual packets. To transmit information they use a TTP that every user and every mix server can access and that stores and provides the following information for every message:
\begin{itemize}
	\item the next hop of a message (if the message has not reached the recipient), or the actual message (if it has reached the recipient).
	\item the next handle $h$
	\item the delay specified by the sender
\end{itemize}
Any protocol participant (users and mix servers) send a series of handles to the TTP whenever they want to send a message. The TTP makes sure that only the recipient of a handle can request the information described above.

\myparagraph{Idea for showing that Game 0 $\approx$ Game 1}
We assume for our analysis that the implementation of the cryptographic primitives underlying the Loopix system is flawless. Moreover we abstract away the computational overhead, space restrictions and communication costs as well as timing channels of clients and mix servers and we assume that there is no network latency other than the delays imposed by Loopix. Moreover, Sphinx does not leak additional information. 
Thus, the adversarial advantage in Game 1 (against the TTP) is equal to the adversarial advantage in Game 0 against Loopix up to a negligible difference (in terms of the security parameter).

\myparagraph{Game 2 (reduced complexity)}
We remove all compromised users from the network (if they should exist). Moreover, we remove all loop messages from mix servers. Thus, only loop messages, drop messages and payload messages from all honest users remain, including the challenge messages. All messages now originate from a client and reach a provider after travelling through the network.

\myparagraph{Idea for showing that Game 1 $\leq$ Game 2}
Compromised users do not contribute to the security of honest users: they can leak their random state to the adversary who can subsequently filter our their messages. Since the idealized version of Loopix does not suffer from space restrictions or computational costs, compromised users do not interfere with honest users. Finally, the adversary does not loose information as it can simulate compromised users locally.

Although we expect mix loops to contribute to the anonymity of honest users against the GPS, their main purpose is to counter active attacks. Since mix loops depend in no way on the challenge of the adversary and since the parameters of mix loops are known, the adversary can also locally simulate mix loops.

Slightly more formally, the transition from Game 1 to Game 2 follows via reduction. Given an adversary \adv against the challenger $\chal_1$ in Game 1, we construct an adversary $\adv'$ against the challenger $\chal_2$ in Game 2 as follows:
$\adv'$ simulates $\adv$ and relays all messages from $\adv$ to the challenger and also relays all network observations to $\adv$. Additionally, $\adv'$ simulates the behavior of all compromised users and generates mix loop messages. It simulates their delays in the network, draws fresh handles for every hop and includes their transmissions in the network observations it relays to $\adv$. 
For compromised mix servers, $\adv$ relays all requests that $\adv$ sends to the TTP, except for requests concerning handles for simulated messages (from compromised users or for mix loops). In those cases, $\adv'$ simulates the answer of the TTP, which it can do, as it simulates those messages itself. Finally, when $\adv'$ outputs its guess $b^*$ for the challenge bit, $\adv$ also outputs $b^*$.

Analyzing the observations that $\adv'$ makes we see that the simulation is perfect. Thus, $\adv'$ cannot change its behavior when simulated by $\adv$. Furthermore, whenever $\adv'$ wins against the simulated Game 1 by guessing $(b^* = b)$ correctly, then $\adv'$ wins against Game 2.

\myparagraph{Game 3 (local computations)}
Instead of the user now every mix node and provider locally chooses the delay and the handle for each message whenever the next hop is a mix node. If the next hop is a provider (i.e., if the message reaches its destination), this provider is specified by the user and stored in the TTP. For all other hops the TTP only receives the handle of a message as well as the next handle. These handles are freshly generated by all mix servers (including honest but curious ones) and the next hop is equally chosen uniformly at random from all available mix nodes for this next hop.

Clients only send the actual message, the recipient (including its provider) and the first handle to the TTP; the TPP then links together this handle and the handles provided by the subsequent mix servers and allows the receiving provider to fetch the message (either a challange message and their recipient or a special symbol indicating a drop message).

\myparagraph{Idea for showing that Game 2 $=$ Game 3}
We only consider passive adversaries. The adversary doesn't control any user's client directly and all remaining users are honest in their choices. Moreover, the providers and mix nodes are honest or, if compromised, honest but curious. Since the adversary cannot access the random choices of the sender of a message, we can make this transition without changing the adversarial advantage. We can show this via a simple reduction. If a mix node / provider is honest, the adversary observes exactly the same. If it is compromised our adversary in the reduction from Game 3 to Game 2 simulates the (richer) responses from the TTP in Game 2 by first drawing the next hop and then appending this choice to the TTP's response.

\myparagraph{Game 4 (simple Loopix)}
The challenger only runs SimpleLoopix, as defined in \Cref{def:simpleloopix}.

\myparagraph{Idea for showing that Game 3 $=$ Game 4}
We show this transition via another reduction. Given an adversary $\adv$ against Game 3, we construct an adversary $\adv'$ against SimpleLoopix.
Since the compromised mix nodes are honest but curious, we assume that they perform their random choices locally and only inform the adversary about them.
$\adv'$ regularly queries the oracles $O_T, O_C$ and $O_M$ for new entries. We note that all transmissions generated by the TTP in SimpleLoopix are generated via the same distribution as transmissions generated in Game 3. Moreover, for all compromised mix nodes, $\adv'$ receives correlated transmissions from $O_C$ and reconstructs the delay between them, which it additionally sends to $\adv$. Finally, when $\adv'$ outputs its guess $b^*$ for the challenge bit, $\adv$ also outputs $b^*$. 
Analyzing the observations that $\adv'$ makes we see that the simulation is perfect. Thus, $\adv'$ cannot change its behavior when simulated by $\adv$. Furthermore, whenever $\adv'$ wins against the simulated Game 3 by guessing $(b^* = b)$ correctly, then $\adv'$ wins against SimpleLoopix.

This concludes the proof.
\end{proof}

We can now proceed to analyze in which cases describe when the adversary can and cannot gain information about the challenge bit of the challenger.

\begin{definition}[Joining traces]
We say that two valid traces $\trace_x = \left ((S_{x_1},h_{x_1},t_{x_1}, R_{x_1}) \ldots (S_{x_l},h_{x_l},t_{x_l}, R_{x_l}) \right)$ and  $\trace_y = \left ((S_{y_1},h_{y_1},t_{y_1}, R_{y_1}) \ldots (S_{y_l},h_{y_l},t_{y_l}, R_{y_l}) \right)$ join at hop $i$ and write $\trace_x \tracejoin{i} \trace_y$ if $R_{x_i} = R_{y_i} \land t_{x_i} < t_{y_{i+1}} \land t_{y_i} < t_{x_{i+1}}$.
\end{definition}

\begin{lemma}[Trace equivalence]\label{lemma:traceequivalence}
Let $m_x, m_y$ be two messages sent by $u_x, u_y$ to $p_x, p_y$ respectively. Moreover let  $\trace_x = \left ((S_{x_1},h_{x_1},t_{x_1}, R_{x_1}) \ldots (S_{x_l},h_{x_l},t_{x_l}, R_{x_l}) \right)$ be any trace generated by $u_x$ sending $m_x$ to $p_x$  and  $\trace_y = \left ((S_{y_1},h_{y_1},t_{y_1}, R_{y_1}) \ldots (S_{y_l},h_{y_l},t_{y_l}, R_{y_l}) \right)$  be any trace generated by $u_y$ sending $m_y$ to $p_y$.

Then if for $i \in \set{2,l-1}$ we have $\trace_x \tracejoin{i} \trace_y$ and we define $\trace_{x-i-y} = ((S_{x_1},\allowbreak h_{x_1}, \allowbreak t_{x_1}, R_{x_1}) \ldots (S_{x_i},h_{x_i},t_{x_i}, R_{x_i}),\allowbreak (S_{y_{i+1}},h_{y_{i+1}},t_{y_{i+1}},\allowbreak R_{y_{i+1}}) \ldots (S_{y_l},h_{y_l},t_{y_l}, R_{y_l}) )$ and $\trace_{y-i-x}$ analogously, then 

\[
\begin{aligned}
&\pr{\trace_x \ot (u_x \overset{m_x}{\rightarrow}p_x) \land \trace_y \ot (u_y \overset{m_y}{\rightarrow}p_y)}\\
=&\pr{\trace_{x-i-y} \ot (u_x \overset{m_y}{\rightarrow}p_y) \land \trace_{y-i-x} \ot (u_y \overset{m_x}{\rightarrow}p_x)}.\\
\end{aligned}
\]
\end{lemma}
\begin{proof}
Let $m_x, m_y$ be two messages sent by $u_x, u_y$ to $p_x, p_y$ respectively, both at time $t_0$. Moreover let  $\trace_x = \left ((S_{x_1},h_{x_1},t_{x_1}, R_{x_1}) \ldots (S_{x_l},h_{x_l},t_{x_l}, R_{x_l}) \right)$ be any trace generated by $u_x$ sending $m_x$ to $p_x$  and  $\trace_y = \left ((S_{y_1},h_{y_1},t_{y_1}, R_{y_1}) \ldots (S_{y_l},h_{y_l},t_{y_l}, R_{y_l}) \right)$  be any trace generated by $u_y$ sending $m_y$ to $p_y$.

Let $i \in \set{2,l-1}$ be s.t. $\trace_x \tracejoin{i} \trace_y$. We define $\trace_{x-i-y} = ((S_{x_1},\allowbreak h_{x_1}, \allowbreak t_{x_1}, R_{x_1}) \ldots (S_{x_i},h_{x_i},t_{x_i}, R_{x_i}),\allowbreak (S_{y_{i+1}},h_{y_{i+1}},t_{y_{i+1}},\allowbreak R_{y_{i+1}}) \ldots (S_{y_l},h_{y_l},t_{y_l}, R_{y_l}) )$ and $\trace_{y-i-x}$ analogously.
Let $P_M(j)$ be the probability distribution over the available mix nodes at the $j$-th layer of Loopix.

We have 
\[
\begin{aligned}
	&\pr{\trace_X \ot u_X \overset{m_X}{\rightarrow}p_X \land \trace_Y \ot u_Y \overset{m_Y}{\rightarrow}p_Y} \\
= 	&\pr{\trace_X \ot u_X \overset{m_X}{\rightarrow}p_X} \cdot \pr{\trace_Y \ot u_Y \overset{m_Y}{\rightarrow}p_Y} \\
= 	& \left(\prod_{j \in \set{2, \ldots, l-1}} \pr{R_{x_j} \ot P_m(j)} \right) \cdot \pr{t_{x_1} - t_0 \ot \Exp(\lambda_P) }\\
& \cdot \left(\prod_{j \in \set{2, \ldots, l}} \pr{t_{x_j} - t_{x_{j-1}} \ot \Exp(\mu) } \right) \\
& \cdot \left(\prod_{j \in \set{2, \ldots, l-1}} \pr{R_{y_j} \ot P_m(j)} \right) \cdot \pr{t_{y_1} - t_0 \ot \Exp(\lambda_P) }\\
& \cdot \left(\prod_{j \in \set{2, \ldots, l}} \pr{t_{y_j} - t_{y_{j-1}} \ot \Exp(\mu) } \right) \\
= 	& \left(\prod_{j \in \set{2, \ldots, l-1}} \pr{R_{x_j} \ot P_m(j)} \right) \cdot \pr{t_{x_1} - t_0 \ot \Exp(\lambda_P) }\\
& \cdot \left(\prod_{j \in \set{2, \ldots, l}\setminus\set{i}} \pr{t_{x_j} - t_{x_{j-1}} \ot \Exp(\mu) } \right) \\
& \cdot \left(\prod_{j \in \set{2, \ldots, l-1}} \pr{R_{y_j} \ot P_m(j)} \right) \cdot \pr{t_{y_1} - t_0 \ot \Exp(\lambda_P) }\\
& \cdot \left(\prod_{j \in \set{2, \ldots, l}\setminus\set{i}} \pr{t_{y_j} - t_{y_{j-1}} \ot \Exp(\mu) } \right) \\
&\cdot \pr{t_{x_i} - t_{x_{i-1}} \ot \Exp(\mu) } \cdot \pr{t_{y_i} - t_{y_{i-1}} \ot \Exp(\mu) }\\
\end{aligned}
\]

Now note that for the probability density functions of \Exp we have:
\[
\begin{aligned}
	&\mathsf{pdf}_{\Exp(\mu)}( t_{x_i} - t_{x_{i-1}} ) \cdot \mathsf{pdf}_{\Exp(\mu)}( t_{y_i} - t_{y_{i-1}} ) \\
=	&\mu e^{-\mu (t_{x_i} - t_{x_{i-1}}) } \cdot \mu e^{-\mu ( t_{y_i} - t_{y_{i-1}} )} \\
=	&\mu^2 e^{-\mu t_{x_i} + \mu t_{x_{i-1}} -\mu  t_{y_i} + \mu t_{y_{i-1}} } \\
=	&\mu e^{-\mu (t_{x_i} - t_{y_{i-1}}) } \cdot \mu e^{-\mu ( t_{y_i} - t_{x_{i-1}} )} \\
=	&\mathsf{pdf}_{\Exp(\mu)}( t_{x_i} - t_{y_{i-1}} ) \cdot \mathsf{pdf}_{\Exp(\mu)}( t_{y_i} - t_{x_{i-1}} ). 
\end{aligned}
\]
Thus, for the probability to draw $t_{x_i} - t_{x_{i-1}}$ and to also draw $t_{y_i} - t_{y_{i-1}}$ we get
\[
\begin{aligned}
	&\pr{t_{x_i} - t_{x_{i-1}} \ot \Exp(\mu) } \cdot \pr{t_{y_i} - t_{y_{i-1}} \ot \Exp(\mu) }\\
=	&\pr{t_{x_i} - t_{y_{i-1}} \ot \Exp(\mu) } \cdot \pr{t_{y_i} - t_{x_{i-1}} \ot \Exp(\mu) }.
\end{aligned}
\]
We use this argument in our calculation and yield 

\[
\begin{aligned}
	&\pr{\trace_X \ot u_X \overset{m_X}{\rightarrow}p_X \land \trace_Y \ot u_Y \overset{m_Y}{\rightarrow}p_Y} \\
= 	& \left(\prod_{j \in \set{2, \ldots, l-1}} \pr{R_{x_j} \ot P_m(j)} \right) \cdot \pr{t_{x_1} - t_0 \ot \Exp(\lambda_P) }\\
& \cdot \left(\prod_{j \in \set{2, \ldots, l}\setminus\set{i}} \pr{t_{x_j} - t_{x_{j-1}} \ot \Exp(\mu) } \right) \\
& \cdot \left(\prod_{j \in \set{2, \ldots, l-1}} \pr{R_{y_j} \ot P_m(j)} \right) \cdot \pr{t_{y_1} - t_0 \ot \Exp(\lambda_P) }\\
& \cdot \left(\prod_{j \in \set{2, \ldots, l}\setminus\set{i}} \pr{t_{y_j} - t_{y_{j-1}} \ot \Exp(\mu) } \right) \\
&\cdot \pr{t_{x_i} - t_{y_{i-1}} \ot \Exp(\mu) } \cdot \pr{t_{y_i} - t_{x_{i-1}} \ot \Exp(\mu) }\\
= 	&\pr{\trace_{x-i-y} \ot u_X \overset{m_X}{\rightarrow}p_X} \cdot \pr{\trace_{y-i-x} \ot u_Y \overset{m_Y}{\rightarrow}p_Y} \\
= 	&\pr{\trace_{x-i-y} \ot u_X \overset{m_X}{\rightarrow}p_X \land \trace_{y-i-x} \ot u_Y \overset{m_Y}{\rightarrow}p_Y} \\
\end{aligned}
\]
\end{proof}

Furthermore, we can combine several joining traces. Thus, we can give a condition on anonymity, depending on the parameters $\lambda_P$ and $\mu$ of Loopix. The probability for the condition to be satisfied additionally depends on $\lambda_D$.

\begin{theorem}[Conditions leading to provable anonymity]
Let $(u_A,u_B,m_C,p_C, m_D,p_D)$ be the challenge sent by the adversary.
Let $H_0 \subseteq \left(\transmissions^l \right)^*$ be the transitions chosen by the challenger (for $b=0$) up to the point in time where the adversary makes its guess for the challenge bit and let $O_T, O_C, O_M$ be the sets provided by the TTP at this time. 
Moreover, let $\trace_C \ot u_A \overset{m_C}{\rightarrow}p_C$ and $\trace_D \ot u_B \overset{m_D}{\rightarrow}p_D$ be the traces the challenger chose for the challenge messages.
Then SimlpeLoopix provides perfect sender-receiver third party anonymity if the following condition holds:
$\exists k \in \mathbb N.\ \exists x_1, \ldots, x_k, y_1, \ldots, y_k \in \set{2, \ldots, l-1}$ and 
$\exists \trace_{x_1}, \ldots, \trace_{x_{l-2}}, \trace_{y_1}, \ldots,  \trace_{y_{l-2}} \in H$, s.t. 
\begin{itemize}
	\item $\forall i \in \set{1, \ldots, k}.$ the traces $\trace_{x_i}$ and $\trace_{y_i}$ are for drop messages.
	\item $\forall i \in \set{1, \ldots, k-1}$ let $(S_x,h_x,t_x,R_x)$ and $(S_y,h_y,t_y,R_y)$ be the transmissions of $\trace_{x_i}$ at position $x_i$ and $\trace_{y_i}$ at position $y_i$ respectively. Then $R_x$ and $R_y$ are not compromised.
	\item $\forall i \in \set{1, \ldots, k-1}.\ x_i < x_{i+1} \land y_i < y_{i+1}$
	\item $\trace_C \tracejoin{x_1} \trace_{x_1} \land  \trace_D \tracejoin{y_1} \trace_{y_1}$
	\item $\forall i \in \set{2, \ldots, k-2}.\ \trace_{x_i} \tracejoin{x_i} \trace_{x_{i+1}} \land \trace_{y_i} \tracejoin{y_i} \trace_{y_{i+1}}$
	\item $\trace_C \tracejoin{y_k} \trace_{y_k} \land  \trace_D \tracejoin{x_k} \trace_{x_k}$.
\end{itemize}
\end{theorem}
\begin{proof}
Note first that all traces $\trace_{a_i}$ and $\trace_{b_j}$ for $a, b \in \set{x,y}$ are traces of drop messages sent by some users to randomly chosen providers. All probabilities for choosing the mixes on the path and for choosing the providers to drop the messages are equal and independent from each other. We leverage \Cref{lemma:traceequivalence} whenever such traces join in a way described in the condition to yield another set $H$ of traces that results in the same observations and that occurs with the same probability as $H_0$.

We then describe a series of hybrid sets of traces $H_{(i,j)}$, where we replace traces using \Cref{lemma:traceequivalence}. Note that all these individual sets of traces occur with the same probability as $H_0$, but under different conditions on the destinations of the challenge messages. Thus, none of the hybrid games necessarily leads to a valid observation. However, after applying \Cref{lemma:traceequivalence} for all $i$ and $j$ successively, we are left with a set $H_1$ that occurs with the same probability as $H_0$, but under the condition that the challenge bit $b=1$ instead of $b=0$. We argue that for different sets of traces $H_0$ we will end up with different sets of traces $H_1$ and we can apply the reasoning in reverse as well and define an ordering on our sets of traces $\set{\trace_{x_1}, \ldots, \trace_{x_k}, \trace_{y_1}, \ldots, \trace_{y_k}}$ to yield an equivalence between each trace in $H_0$ and exactly one trace in $H_1$. 

We argue that whenever the TTP in the challenge response game produces a set of traces $H_0$ for which our condition is fulfilled, the adversarial advantage necessarily is $0$, as there is exactly one $H_1$ leading to the same observation $(O_T,O_C,O_M)$ and having the same probability to occur for the challenge bit $b=1$ than $H_0$ has for $b=0$.
\end{proof}
\myparagraph{Quantification}
\[
	\sim
\]
